# Supplementary material for: Conversation Model Fine-Tuning for Classifying Client Utterances in Counseling Dialogues
Source: arXiv:1904.00350 source file (2019-03-31)
Supplement: Supplementary file 1 [file Appendix.tex]

\section*{Appendix}

\begin{table}[!h]
\centering
\small
\begin{tabular}{ c | m{6cm} | m{6cm} }
\toprule
\multicolumn{1}{l|}{} & \multicolumn{1}{c|}{\textbf{Counselor}} & \multicolumn{1}{c}{\textbf{Client}} \\ \midrule
\multirow{5}{*}{\textbf{\begin{tabular}[c]{@{}c@{}}Factual \\ Information\end{tabular}}} & nice to meet you & never visited neuropsychiatry \\
 & of course first & female , worker \\
 & I see. now & \small{never received psychological counseling} \\
 & . . {[}client's name{]}'s & motivation of counseling \\
 & well . . & age \# , female \\ \midrule
\multirow{5}{*}{\textbf{\begin{tabular}[c]{@{}c@{}}Anecdotal\\ Experience\end{tabular}}} & might be left behind & too hard \\
 & be in a peer relationships & didn't get along \\
 & I see. actually & seem to be \\
 & well . . & I thought that \\
 & I understand what you mean & I was totally wrong \\ \midrule
\multirow{5}{*}{\textbf{\begin{tabular}[c]{@{}c@{}}Appealing\\ Problem\end{tabular}}} & right . all & sick and sad \\
 & but now the relationship is & have many thoughts \\
 & nice to meet you & keep thinking \\
 & you told me well & I think I did it \\
 & more comfortable? & no future and frustrating \\ \midrule
\multirow{5}{*}{\textbf{\begin{tabular}[c]{@{}c@{}}Psychological\\ Change\end{tabular}}} & right . and & did not think so but \\
 & if you do that someday & I was so shocked \\
 & suddenly I did & it could have been longer \\
 & I hope so & but looking back \\
 & question arises & I think I will \\ \midrule
\multirow{5}{*}{\textbf{\begin{tabular}[c]{@{}c@{}}Counseling\\ Process\end{tabular}}} & hard to express but & how are you ? \\
 & counseling proceeds & what do you think ? \\
 & Hello ? {[}client's name{]} , & thank you for listening \\
 & let's talk at \# & hello counselor \\
 & yes the counseling time is & time is not enough \\ \bottomrule
\end{tabular}
\caption {Representative phrases in utterances of both conversational parties, extracted based on the relative importance of the phrase in terms of classification by using attention weights.}
\label{table:qual}
\end{table}
